# Supplementary material for: BlinkML: Efficient Maximum Likelihood Estimation with Probabilistic Guarantees
Source: arXiv:1812.10564 source file (2018-12-26)
Supplement: Supplementary file 1 [file additional_exp.tex]

\section{Additional Experiments}
\label{sec:add:exp}

\input{figures/fig_hyperparam}

\input{figures/fig_exp_model_complexity}

\subsection{Hyperparameter Optimization}

\tofix{
This section studies \system's benefits in hyperparameter optimization.
Specifically, we compared the accuracies of the models (with different feature sets and hyperparameters) trained by \system and a regular system.
As performed by Random Search~\cite{bergstra2011algorithms},
we first generated a sequence of (pairs of) a randomly chosen feature set and a regularization coefficient.
Then, we let \system train a series of 95\% accurate models using the feature set and the regularization coefficient in the sequence.
Similarly, we let the regular system train a series of exact models using the same combination of the feature set and the regularization coefficient.

\cref{fig:exp:hyperparam} shows the result. Each dot in the figure represents a model. In half an hour, \system trained 961 models while the regular system trained only 3 models.
\system found the second-best model (with test accuracy 74\%; found at iteration \#2) in 1.03 seconds, while the regular system took 817 seconds until it trains the second-best model. In 387 seconds, \system found the best model (with test accuracy 75\%; found at iteration \#91).
The sizes of the samples used by \system varied between 10,000 and 9,211,426, depending on the feature set and the regularization coefficient. Note that this is an expected behavior since \system automatically chooses the sample size that is large enough to produce an accurate model. We study this behavior more systematically in the following section.
}

\subsection{Impact of Model Complexity on Estimated Sample Sizes}
\label{sec:exp:model}

\tofix{
We also studied the impact of model complexity on \system's estimated sample size.
Intuitively, if a model is more complex, a larger sample would be needed for training an accurate model (i.e., the model highly similar to the full model). To control the complexity of a model, we varied the regularization coefficient and the number of parameters (i.e., the number of features) of the model. We used LR for this experiment.

\cref{fig:exp:model} shows the results.
On the left (\cref{fig:exp:model:a}), we can see that as the model became less complex (or more rigid with a larger regularization coefficient), the estimated sample size decreased.
On the right (\cref{fig:exp:model:b}), we can see that as the model became more complex (with a larger number of parameters), the estimated sample size increased.
These results demonstrate the adaptive nature of \cref{thm:param_dist}, which \system relies on for estimating sample sizes.
}
