# Supplementary material for: BlinkML: Efficient Maximum Likelihood Estimation with Probabilistic Guarantees
Source: arXiv:1812.10564 source file (2018-12-26)
Supplement: Supplementary file 2 [file appendix_discussion.tex]

%!TEX root = approx_ml.tex

\section{Small Sample Sizes and High-Dimensional Data}
\label{sec:appendix:discussion}

\cref{thm:param_dist} and \cref{thm:cond_param_dist} use asymptotic distributions (as $n \rightarrow \infty$) for characterizing the relationship between the approximate model's parameters (i.e., $\theta_n$) and the (unknown) full model's model parameters (i.e., $\hat{\theta}_N$). In practice, this relationship 
can be characterized  more accurately as long as $n$ is \emph{not} too small (i.e., $n$ > 100). In our typical use-cases, the value of $n$ is at least several thousands (10,000 by default), and $N$ is typically over a million.

Furthermore, $H$ and $J$ in \cref{thm:param_dist} and \cref{thm:cond_param_dist} are both $d$-by-$d$ matrices, where $d$ is the dimension of training examples, i.e., their space requirement  is $O(d^2)$. 
Our current technique can therefore handle many common BI scenarios (e.g., TPC-H~\cite{tpch_website}, TPC-DS~\cite{tpcds_website}, Instacart~\cite{instacart_website}, Dunnhumby~\cite{dunnhumby_website}), where joined tables have several hundreds of columns. For instance, our experiments in \cref{sec:exp} include   datasets with up to 1,000 features. 
However, to support extremely high-dimensional scenarios (i.e., $d$ being over a million) our current approach needs to be extended, so that it can  avoid explicit materialization of $H$ and $J$. We leave this as future work.
