# Supplementary material for: BlinkML: Efficient Maximum Likelihood Estimation with Probabilistic Guarantees
Source: arXiv:1812.10564 source file (2018-12-26)
Supplement: Supplementary file 3 [file additional_experiment.tex]

% \input{exp_statistics}
